# Supplementary material for: PopSim: An Individual-level Population Simulator for Equitable Allocation of City Resources
Source: arXiv:2305.02204 source file (2023-04-25)
Supplement: Supplementary file 1 [file appendixA.tex]

\appendix
\onecolumn

\section{Appendix: Graphs for the average distance for each race to reach to the nearest resource}\label{sec:appendixA}

\begin{figure}[H]
\begin{subfigure}{.5\textwidth}
  \centering
  \includegraphics[width=\linewidth]{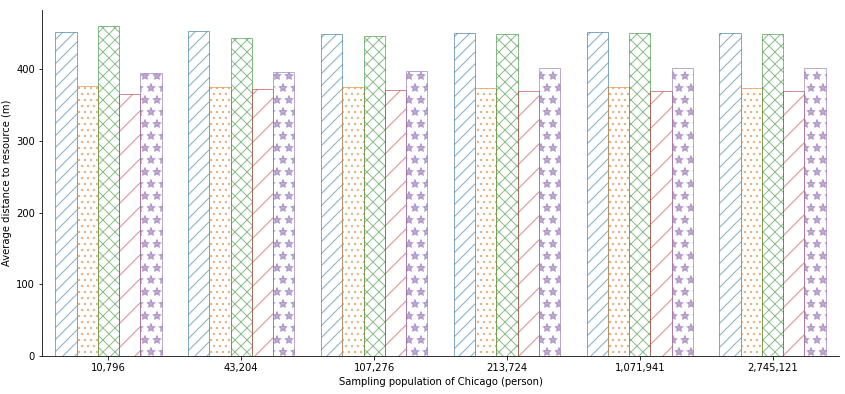}
  \caption{Schools}
  \label{fig:sfig1}
\end{subfigure}%
\begin{subfigure}{.5\textwidth}
  \centering
  \includegraphics[width=\linewidth]{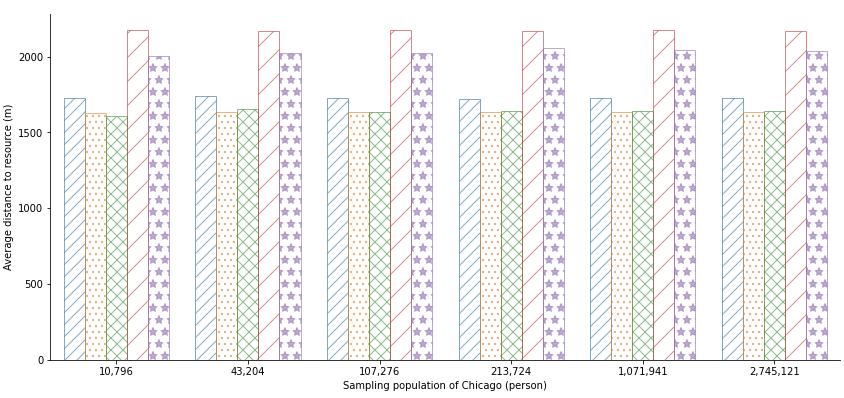}
  \caption{Hospitals}
  \label{fig:sfig2}
\end{subfigure}
\begin{subfigure}{.5\textwidth}
  \centering
  \includegraphics[width=\linewidth]{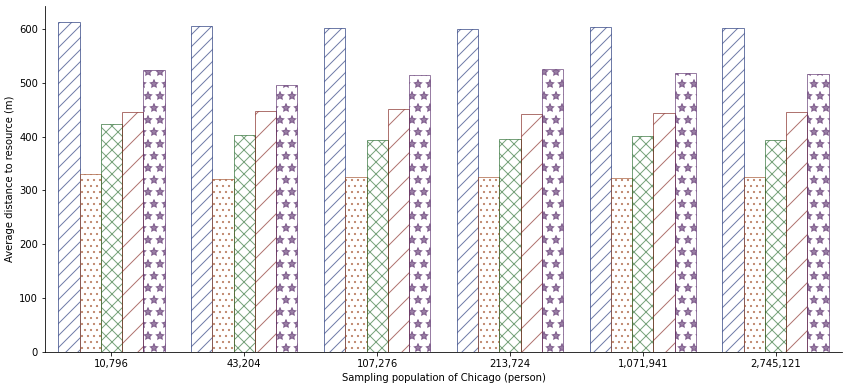}
  \caption{Divvy bike stations}
  \label{fig:sfig2}
\end{subfigure}
\begin{subfigure}{.5\textwidth}
  \centering
  \includegraphics[width=\linewidth]{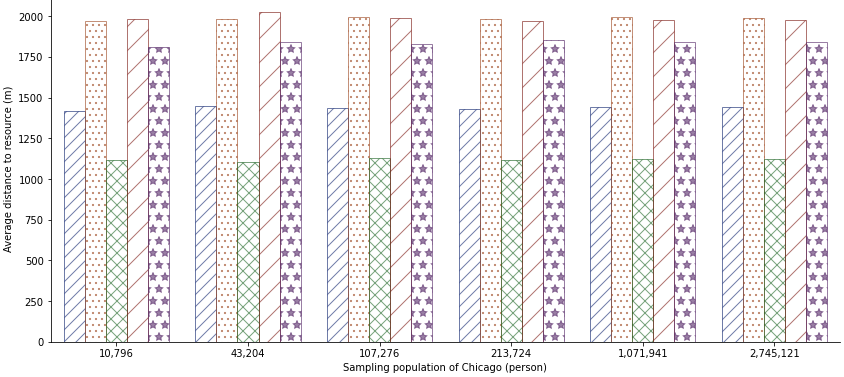}
  \caption{CTA train stations}
  \label{fig:sfig2}
\end{subfigure}
\begin{subfigure}{.5\textwidth}
  \centering
  \includegraphics[width=\linewidth]{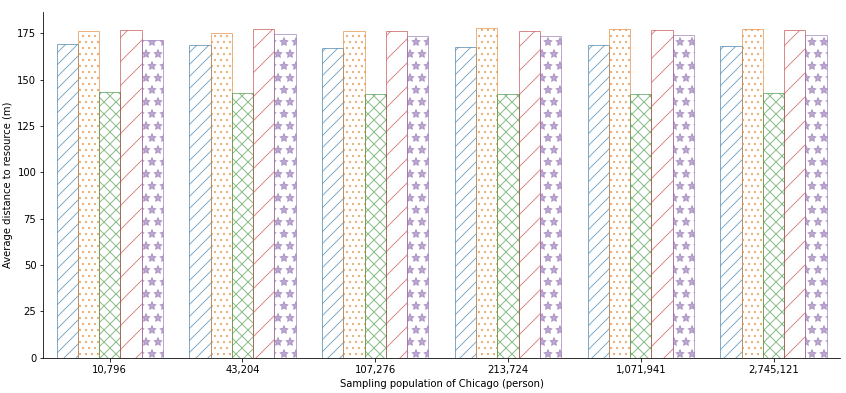}
  \caption{Bus stops}
  \label{fig:sfig2}
\end{subfigure}
\begin{subfigure}{0.5\textwidth}
  \centering
  \hspace{-60mm}
  \vspace{30mm}
  \includegraphics[width=0.2\linewidth]{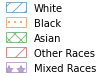}
  \label{fig:sfig2}
\end{subfigure}
\end{figure}
